# Supplementary material for: Normative Modules: A Generative Agent Architecture for Learning Norms that Supports Multi-Agent Cooperation
Source: arXiv:2405.19328 source file (2024-05-29)
Supplement: Supplementary file 1 [file 8_appendix.tex]

\section{Appendix}
\begin{figure}{R}{0.5\textwidth}

  \centering
  \includegraphics[width=0.5\textwidth]{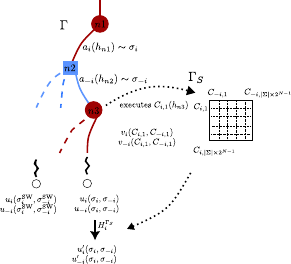} % Adjust the width as needed
  \caption{Sanction-based transformation of an extensive form game $\Gamma$ through a sanction game $\Gamma_{S}$}
  \label{fig:game_transformation} % You can use this label to reference the figure

\end{figure}
\begin{theorem}
Any arbitrary strategy $(\sigma_{i},\sigma_{-i})$ in $\Gamma$ can be can be transformed into a Nash equilibrium under a sanction-based transform $H^{\Gamma_{S}^{\infty}}$ with an infinitely repeated sanction game $\Gamma_{S}^{\infty}$ when $\underbar{v}_{i} < \Delta_{i}$. Here $\Delta_{i}$ can be expressed as $\sum\limits_{C \in 2^{\Sigma}} \alpha_{C} v_{i}(C_{i},C_{-i})$ with $\sum \alpha_{C} = 1$, where $\Delta_{i} = u_{i}(BR(\sigma_{-i}),\sigma_{-i}) - u_{i}(\sigma_{i},\sigma_{-i})$ and $\underbar{v}_{i}$ is the minimax payoff of $\Gamma_{S}^{\infty}$.
\end{theorem}
\begin{proof}
We first characterize the set of equilibrium payoffs in the sanction game infinitely repeated game $\Gamma_{S}^{\infty}$ under average utilities. Note that the space of actions in $\Gamma_{S}$ is $2^{\Sigma}$ corresponding to the all classification functions over the space of strategy profiles $\Sigma$ in the original game $\Gamma$.\par
Let 
\begin{equation*}
    \underbar{v}_{i} = \min\limits_{C_{-i} \in 2^{\Sigma}} \max\limits_{C_{i} \in 2^{\Sigma}} v_{i}(C_{i},C_{-i})
\end{equation*}
be the minimax value of the player in the game $\Gamma_{S}$. By the Folk theorem, any payoff profile $v_{i}^{*}$ in the repeated game $\Gamma_{S}^{\infty}$ played infinitely often can be supported in Nash equilibrium iff $\forall i \in N$, $v_{i}^{*} > \underbar{v}_{i}$ (enforceable condition) and there exists rational values $\alpha_{C}$ such that $\forall C_{-i}$, $\forall i$, $v_{i}^{*}$ can be expressed as $\sum\limits_{C \in 2^{\Sigma}} \alpha_{C} v_{i}(C_{i},C_{-i})$ with $\sum \alpha_{C} = 1$.\par
Take any arbitrary strategy profile $\sigma_{i},\sigma_{-i}$ in $\Gamma$. If they are not in Nash equilibria, then $BR_{i}(\sigma_{-i}) \neq \sigma_{i}$ and/or $BR_{-i}(\sigma_{i}) \neq \sigma_{-i}$, where $BR$ is the Best Response function.\par
Let $\Delta_{i} = u_{i}(BR(\sigma_{-i}),\sigma_{-i}) - u_{i}(\sigma_{i},\sigma_{-i})$ be the deviation incentive for $i$ in the strategy profile $(\sigma_{i},\sigma_{-i})$. Similarly ($\Delta = \Delta_{i},\Delta_{-i}$) is the vector of incentive deviation for all players in the strategy profile. The transform $H^{*}_{i}(u_{i}(\sigma_{i},\sigma_{-i})) = u_{i}'(\sigma_{i},\sigma_{-i})$ induced by the equilibrium utilities (cost) of $\Gamma_{S}^{\infty}$ can be written as follows:
\begin{align}
     u_{i}'(\sigma_{i},\sigma_{-i}) &= u_{i}(\sigma_{i},\sigma_{-i}) - v_{i}(C_{i}^{*}(\sigma_{i}), C_{-i}^{*}(\sigma_{-i})) \\
     &= u_{i}(BR(\sigma_{-i}),\sigma_{-i}) - (u_{i}(BR(\sigma_{-i}),\sigma_{-i}) - u_{i}(\sigma_{i},\sigma_{-i})) - v_{i}^{*}(C_{i}^{*}(\sigma_{i}), C_{-i}^{*}(\sigma_{-i})) \\
     &= u_{i}(BR(\sigma_{-i}),\sigma_{-i}) - \Delta_{i} - v_{i}^{*}(C_{i}^{*}(\sigma_{i}), C_{-i}^{*}(\sigma_{-i}))
\end{align}
setting the condition that 
\begin{equation}
    v_{i}^{*}(C_{i}^{*}(\sigma_{i}), C_{-i}^{*}(\sigma_{-i})) = -\Delta_{i}
\end{equation}
Eqn 4 leads to the following equality
\begin{equation*}
    u_{i}'(\sigma_{i},\sigma_{-i}) = u_{i}(BR(\sigma_{-i}),\sigma_{-i})
\end{equation*}
Therefore, in the transformed utility $\forall i$, there is no incentive to deviate in the strategy profile $(\sigma_{i},\sigma_{-i})$, thereby establishing the Nash equilibrium condition under the transformation.
\end{proof}

\subsection{Compute Resources Used}
\label{compute_resources}

All of our experiments are run on a single GPU node containing four A40 nvidia GPUs, 32 CPU cores, and 167 Gb of RAM.
